# Supplementary material for: Leveraging Procedural Knowledge and Task Hierarchies for Efficient Instructional Video Pre-training
Source: arXiv:2502.17352 source file (2025-02-24)
Supplement: Supplementary file 1 [file appendix.tex]

\appendix
\section{Additional Experimental Results}

We also test which subset of the hierarchy path labels to use in pre-training. We observe that using the first two levels...
